# Supplementary material for: Separation and Encodability in Mixed Choice Multiparty Sessions (Technical Report)
Source: arXiv:2405.08104 source file (2024-06-07)
Supplement: Supplementary file 1 [file app-subtyping.tex]

\section{Mixed choice session subtyping}

\subsection{Proof for Proposition~\ref{prop:subtyping_properties}}
\propsubtyping*

\begin{proof}
	\hfill
	\begin{enumerate}
		\item	{\bf Part 1:} We need to show that $\locali{1} \subt \locali{2}$ is reflexive and transitive.

				The proof for reflexivity is a straightforward induction on the definition of \subt.
				We provide a characteristic case.
				\[
					\Tor{i \in I} \tout{\p}{\lab_i} \locali{i} \subt \Tor{i \in I} \tout{\p}{\lab_i} \locali{i}
				\]
				since $I \subseteq I$ and from the induction hypothesis, it holds that $\forall i \in I, \locali{i} \subt \locali{i}$.

				The proof for transitivity is done by induction on the definition of $\subt$.
				We provide a characteristic case.
				
				Assume
				\begin{eqnarray}
					\Tor{i \in I} \tout{\p}{\lab_i} \locali{i} &\subt& \Tor{j \in J} \tout{\p}{\lab_j} \localid{j}
					\label{app:proof:subtyping_properties:eq1}
					\\
					\Tor{j \in J} \tout{\p}{\lab_j} \localid{j} &\subt& \Tor{k \in K} \tout{\p}{\lab_k} \localidd{k}
					\label{app:proof:subtyping_properties:eq2}
				\end{eqnarray}
				Result~\ref{app:proof:subtyping_properties:eq1} and rule \SSel imply
				\begin{eqnarray}
					\tree {
						J \subseteq I \qquad \forall j \in J, \locali{j} \subt \localid{j}
					}{
						\Tor{i \in I} \tout{\p}{\lab_i} \locali{i} \subt \Tor{j \in J} \tout{\p}{\lab_j} \localid{j}
					}{}
					\label{app:proof:subtyping_properties:eq3}
				\end{eqnarray}
				Moreover, result~\ref{app:proof:subtyping_properties:eq1} and rule \SSel imply
				\begin{eqnarray}
					\tree {
						K \subseteq J \qquad \forall k \in k, \localid{k} \subt \localidd{k}
					}{
					\Tor{j \in J} \tout{\p}{\lab_j} \localid{j} \subt \Tor{k \in K} \tout{\p}{\lab_k} \localidd{k}
					}{}
					\label{app:proof:subtyping_properties:eq4}
				\end{eqnarray}
				Results~\ref{app:proof:subtyping_properties:eq3} and~\ref{app:proof:subtyping_properties:eq4} we get
				\begin{eqnarray*}
					K \subseteq J \subseteq I &\implies& K \subseteq I
					\\
					\forall k \in K, \locali{k} \subt \localidd{k} && \text{from Induction Hypothesis}
				\end{eqnarray*}
				We can then conclude
				\begin{eqnarray*}
					\tree {
						K \subseteq I \qquad \forall k \in k, \locali{k} \subt \localidd{k}
					}{
						\Tor{i \in I} \tout{\p}{\lab_i} \locali{i} \subt \Tor{k \in K} \tout{\p}{\lab_k} \localidd{k}
					}{}
				\end{eqnarray*}
				as required.

		\item {\bf Part 2:} The prove that $\LLi{1} \subt \LLi{2}$ is reflexive and transitive, is straightforward by the definition of $\subt$ and
		Part 1.
		
		Reflexive: it holds that
		\[
			\set{\p_i: \locali{i}}_{i \in I} \subt \set{\p_i: \locali{i}}_{i \in I}
		\]
		since $\forall i \in I, \locali{i} \subt \locali{i}$ (reflexivity of \subt for local types).

		Transitive: assume
		\begin{eqnarray*}
			\set{\p_i: \locali{i}}_{i \in I} &\subt& \set{\p_i: \localid{i}}_{i \in I}
			\\
			\set{\p_i: \localid{i}}_{i \in I} &\subt& \set{\p_i: \localidd{i}}_{i \in I}
		\end{eqnarray*}
		From the reflexitivity of \subt for local types, we have
		\[
			\forall i \in I, \locali{i} \subt \localidd{i}
		\]
		It is then straightforward to imply
		\begin{eqnarray*}
			\set{\p_i: \locali{i}}_{i \in I} &\subt&  \set{\p_i: \localidd{i}}_{i \in I}
		\end{eqnarray*}
		from the definition of $\subt$ for local contexts.

		\item {\bf Part 3:} \dk{TODO}
	\end{enumerate}
\end{proof}
